# Supplementary material for: Smooth Fictitious Play in Stochastic Games with Perturbed Payoffs and Unknown Transitions
Source: arXiv:2207.03109 source file (2022-07-07)
Supplement: Supplementary file 1 [file c_stochastic_approximations.tex]

{
    \NewDocumentCommand{\sax}{}{y}

\begin{theorem}\label{thm:asyncapprox}
    Suppose that:
    \begin{enumerate}[label=(\roman*)]
        \item $\sax_n \in C$ for all $n$ where $C$ is compact
        \item The set valued application $F:C \rightrightarrows C$ is Marchaud
        \item Sequence $\gamma_n$ is such that \begin{enumerate}
            \item $\sum_n \gamma_n = \infty$ and $\gamma_n \xrightarrow[n\rightarrow \infty]{} 0$
            \item for $x \in(0, 1), \sup_n \gamma_{\left[xn\right]}/\gamma_n < A_x < \infty$ where $\left[\cdot \right]$ is the floor function.
            \item for all $n$, $\gamma_n \geq \gamma_{n+1}$
        \end{enumerate}
        \item \begin{enumerate}
            \item For all $\sax\in C$, $\mathcal S_n, \mathcal S_{n+1} \in \mathcal S$,
            $\mathbb P(S_{n+1} = \mathcal S_{n+1}|\mathcal F_n)= \\ \mathbb P(S_{n+1}=\mathcal S_{n+1}|S_n = \mathcal S_n, \sax_n=\sax)$
            \item The probability transition between $\mathcal S_n$ and $\mathcal S_{n+1}$ is Lipsichitz continuous in $x_n$ and the Markov chain that $S_n$ form is aperiodic, irreducible and for every $s \in \mathcal S$, there exists $S \in \mathcal S$ such that $s \in S$.
        \end{enumerate}
        \item For all $n$, $Y_{n+1}$ and $S_{n+1}$ are uncorrelated given $\mathcal F_n$
        \item For some $q \geq 2$, $\left\{\begin{aligned}&\sum_n \gamma_n^{1+q/2} < \infty \\ & \sup_n \mathbb E(\|Y_n\|^q)<\infty\end{aligned}\right.$
        \item $d_n\rightarrow 0$ when $n\rightarrow \infty$
        
    \end{enumerate}
    Then with probability 1, affine interpolation $\overline \sax$ is an asymptotic pseudo-trajectory to the differential inclusion,
    $$\diff \sax \in \overline F(\sax)$$
    where $\left\{
      \begin{aligned}
        &\overline F(\sax) := \Omega^\epsilon_{k, \sigma} \cdot F(\sax)\\
        & \Omega^\epsilon_k := 
        \left\{\text{diag}(\beta_1, \ldots, \beta_k)
          \left|
            \begin{aligned}
              \forall i \in \left\{1, \ldots, k\right\}, \\
              \beta_i \in [\epsilon, 1]
            \end{aligned}
          \right.
        \right\} \\
        & \epsilon > 0
      \end{aligned}\right.$
    \end{theorem}

}
